# Supplementary material for: VecGAN: Image-to-Image Translation with Interpretable Latent Directions
Source: arXiv:2207.03411 source file (2022-07-07)
Supplement: Supplementary file 1 [file additional_exp.tex]

\begin{table*}[t]
    \centering
    \resizebox{\textwidth}{!}{
    \begin{tabular}{|l|l|l|l|l|}
\hline
\multicolumn{1}{|c|}{\multirow{2}{*}{\textbf{Configuration}}} & \multicolumn{2}{c}{\textbf{Realism FID}}                                                                  & \multicolumn{2}{c|}{\textbf{Disentanglement FID}}                                                         \\ \cline{2-5} 
\multicolumn{1}{|c|}{}                                        & \multicolumn{1}{c}{\textbf{Latent-guided}} & \multicolumn{1}{c|}{\textbf{Reference Guided}} & \multicolumn{1}{c}{\textbf{Latent-guided}} & \multicolumn{1}{c|}{\textbf{Reference Guided}} \\ \hline
SDIT \cite{wang2019sdit} & 33.73 & 33.12 & 80.25 & 79.72\\
StarGANv2 \cite{starganv2} & 26.04 & 25.49 & 90.08 & 78.03\\
HiSD \cite{li2021image} &  21.37 &  21.49 &  71.85 & 71.48 \\

HiSD 128x128(trained)  &  21.35 & 22.55 & 71.69 & 72.94 \\
v1 - Single Discriminator & 26.27 & 26.84 & 78.15 & 78.36 \\
v2 - Double Discriminator & 27.18 & 26.38 & 79.45 & 77.77 \\
v3 - Self translation (170k) & 26.49 & 26.33 & 77.70 & 77.93 \\
v4 - Deeper encoder/decoder (120k) & 24.08 & 24.19 & 74.71 & 75.03\\
v4 - Deeper encoder/decoder (150k) & 23.69 & 23.76 & 75.23 & 74.74 \\
v4 - Deeper encoder/decoder (190k) & 23.70 & 23.53 & 74.09 & 74.15 \\
v4 - Deeper encoder/decoder (200k) & 26.27 & 26.49 & 76.16 & 76.74 \\
v5 - Skip connections (70k) & 23.93 & 23.59 & 74.70 & 74.27 \\
v5 - Skip Connections (160k) & 25.52 & 24.99 & 76.52 & 76.03 \\
v6 - Shift discriminator (160k) & 24.97 & 25.15 & 77.64 & 77.87 \\
v6 - Shift discriminator (200k) & 25.07 & 23.71 & 77.34 & 75.30 \\
v7 - no skip connections - 8x8 & 37.31 & 29.55 & 86.13 & 78.03 \\
v8 (128-8x8) - Attention skip (110k) & 24.11 & 23.39 & 75.42 & 73.69 \\
v8 (256-8x8) - Attention skip (100k) & 23.15 & 23.17 & 74.29 & 74.03 \\
v9 - Learnable orthagonality (200k) & 23.25 & 23.50 & 73.66 & 73.66 \\
v9 - Shift discriminator (alpha + tag) (270k) & 21.75 & 21.74 & 73.16 & 73.06 \\

\hline
\end{tabular}}
    \caption{Evaluation results for experiments}
    \label{tab:HiSD results}
\end{table*}

\begin{table*}[t]
    \centering
    \resizebox{\textwidth}{!}{
    \begin{tabular}{|l|l|l|l|l|}
\hline
\multicolumn{1}{|c|}{\multirow{2}{*}{\textbf{Iteration}}} & \multicolumn{2}{c}{\textbf{Realism FID}}                                                                  & \multicolumn{2}{c|}{\textbf{Disentanglement FID}}                                                         \\ \cline{2-5} 
\multicolumn{1}{|c|}{}                                        & \multicolumn{1}{c}{\textbf{Latent-guided}} & \multicolumn{1}{c|}{\textbf{Reference Guided}} & \multicolumn{1}{c}{\textbf{Latent-guided}} & \multicolumn{1}{c|}{\textbf{Reference Guided}} \\ \hline
90k & 24.18 & 23.03 & 75.67 & 73.82 \\
100k & 23.07 & 23.12 & 74.36 & 73.76 \\
110k & 23.47 & 23.48 & 74.68 & 74.59 \\
120k & 24.69 & 24.57 & 76.22 & \\
200k & 24.46 & 24.14 & 75.34 & 75.21\\
\end{tabular}}
    \caption{Evaluation over iterations for the optimum model (256-8x8) - Attention skip (100k)}
    \label{tab:over_iters}
\end{table*}

\begin{table}[t]
    \centering
    \begin{tabular}{|l|l|l|l|l|}
\hline
\multicolumn{1}{|c|}{\multirow{2}{*}{\textbf{Configuration}}} & \multicolumn{2}{c}{\textbf{Realism}}                                                                  & \multicolumn{2}{c|}{\textbf{Disentanglement}}                                                         \\ \cline{2-5} 
\multicolumn{1}{|c|}{}                                        & \multicolumn{1}{c}{\textbf{L}} & \multicolumn{1}{c|}{\textbf{R}} & \multicolumn{1}{c}{\textbf{L}} & \multicolumn{1}{c|}{\textbf{R}} \\ \hline
HiSD \cite{li2021image} &  21.37 &  21.49 &  71.85 & 71.48 \\
HiSD (32x32)  &  21.35 & 22.55 & 71.69 & 72.94 \\
HiSD (16x16)   \\
HiSD (8x8)  \\
HiSD (4x4)  \\
\hline
\end{tabular}
    \caption{Evaluation results for experiments}
    \label{tab:HiSD_abl}
\end{table}

\begin{table}[t]
    \centering
    \begin{tabular}{|l|l|l|l|l|}
\hline
\multicolumn{1}{|c|}{\multirow{2}{*}{\textbf{Configuration}}} & \multicolumn{2}{c}{\textbf{Realism}}                                                                  & \multicolumn{2}{c|}{\textbf{Disentanglement}}                                                         \\ \cline{2-5} 
\multicolumn{1}{|c|}{}                                        & \multicolumn{1}{c}{\textbf{L}} & \multicolumn{1}{c|}{\textbf{R}} & \multicolumn{1}{c}{\textbf{L}} & \multicolumn{1}{c|}{\textbf{R}} \\ \hline

Ours (32x32)  & 26.27 & 26.84 & 78.15 & 78.36  \\
Ours (16x16) & 23.70 & 23.53 & 74.09 & 74.15   \\
Ours (8x8)  \\
Ours (4x4)  \\
\hline
\end{tabular}
    \caption{Evaluation results for experiments}
    \label{tab:ours_abl}
\end{table}
